# Supplementary material for: The Art of CPU-Pinning: Evaluating and Improving the Performance of Virtualization and Containerization Platforms
Source: arXiv:2006.02055 source file (2020-06-03)
Supplement: Supplementary file 1 [file sec-apndx.tex]

\section{Appendix}\label{sec:apndx}

\begin{lemma}
\label{LeftCosetsDisjoint}
Let $N$, $C(k)$, and $S(k)$ be the total number of network nodes, compromised set of nodes, and secure (non-compromised) network nodes, respectively. Also, we define $V$ and $\beta(k)$ to be, respectively, the vulnerability factor, and the number of network nodes which get compromised at the $k$-th step during the MDP generation phase. 
Then
\begin{equation}
\beta(k+1) = N\cdot\big(\frac{N-V}{N}\big)^{\frac{\log(1-\frac{C(k)}{N})}{\log(\frac{N-V}{N})}}\cdot\Big[ 1 - \big(\frac{N-V}{N}\big)^{\beta(k)} \Big],
\end{equation}

\end{lemma}

\begin{IEEEproof}
Clearly, the number of internal compromised network nodes is initially zero, i.e., $C(0) = 0$. Given the vulnerability factor of $V$, the next step of the MDP generation will result in $C(1) = V$, i.e., $V$ new MDP states. Next, \name will use each of the $V$ compromised nodes, and the non-compromised hosts which are accessible from any of those $V$ compromised nodes, to further expand the MDP model. It is important to mention that exploration of every compromised node will result in $\leq V$ new compromised nodes as some them may have already been compromised during one of the previous steps. 

We calculate the expected number of non-compromised network nodes which are visited (get compromised) at the $k$-th step of the MDP generation procedure, i.e., $\beta(k+1)$. Clearly, those network nodes are visited through investigation of the nodes which got newly compromised during the previous phase $\beta(k)$. Once the first node out of the $\beta(k)$ nodes is investigated, the expected number of compromised nodes is $E[c_k(1)] = C(k) + V\cdot\frac{N-C(k)}{N}$, where $V\cdot\frac{N-V}{N}$ new nodes are compromised, because $V$ (vulnerability factor) nodes are selected which are each non-compromised with probability $\frac{N-V}{N}$. Following some algebraic calculations and arrangements, we have the closed form solution 
\begin{equation}
c_0(n) = N\cdot\Big[1-\big(\frac{N-V}{N}\big)^{n}\Big],
\end{equation}
and hence, we calculate $\beta(k+1)$ as $C(k+1) - C(k)$:
\begin{equation}
\beta(k+1) = N\cdot\big(\frac{N-V}{N}\big)^\alpha\cdot\Big[ 1 - \big(\frac{N-V}{N}\big)^{\beta(k)} \Big],
\end{equation}
where
\begin{equation}
\alpha = \frac{\log(1-\frac{C(k)}{N})}{\log(\frac{N-V}{N})}.
\end{equation}

\qed
\end{IEEEproof}
