# Supplementary material for: The Art of CPU-Pinning: Evaluating and Improving the Performance of Virtualization and Containerization Platforms
Source: arXiv:2006.02055 source file (2020-06-03)
Supplement: Supplementary file 2 [file sec-appendix.tex]

%\section*{}

\begin{wrapfigure}{r}{0.17\textwidth}
  \begin{center}
    \includegraphics[width=0.15\textwidth]{./Figures/saman-zonouz}
  \end{center}
\end{wrapfigure}

\noindent\textbf{Saman Zonouz} is an Assistant Professor in the Electrical and Computer Engineering Department at the University of Miami. He received his Ph.D. in Computer Science from the University of Illinois at Urbana-Champaign in 2011. He has worked on intrusion response and recovery, information flow-based security metrics for power-grid critical infrastructures, online digital forensics analysis and monitorless recoverable applications. His research interests include: computer security and survivable systems, control/game theory, intrusion response and recovery systems, automated intrusion forensics analysis, and information flow analysis-based security metrics.

\begin{comment}
\begin{wrapfigure}{r}{0.17\textwidth}
  \begin{center}
    \includegraphics[width=0.14\textwidth]{./Figures/matt-davis}
  \end{center}
\end{wrapfigure}
\end{comment}

\noindent\textbf{Charles M. Davis} received the B.S. degree in electrical engineering from Louisiana Tech University in 2002 and the M.S. and Ph.D. degrees from the Electrical and Computer Engineering Department at the University of Illinois at Urbana-Champaign.  He is currently working at PowerWorld Corporation.  His research interests include linear sensitivities, power system analysis, power system visualization, and power system operational reliability.

\begin{comment}
\begin{wrapfigure}{r}{0.17\textwidth}
  \begin{center}
    \includegraphics[width=0.14\textwidth]{./Figures/kate-davis}
  \end{center}
\end{wrapfigure}
\end{comment}

\noindent\textbf{Katherine R. Davis} received the B.S. degree in electrical engineering from the University of Texas at Austin in 2007 and the M.S. and Ph.D. degrees from the University of Illinois Urbana-Champaign in 2009 and 2011. She is a software engineer and senior consultant at PowerWorld Corporation and an Adjunct Assistant Professor in Electrical and Computer Engineering Department at the University of Illinois Urbana-Champaign. Her research interests include data-enhanced power system modeling and analysis and making the grid more robust with respect to bad data.

\begin{wrapfigure}{r}{0.17\textwidth}
  \begin{center}
    \includegraphics[width=0.14\textwidth]{./Figures/robin-berthier}
  \end{center}
\end{wrapfigure}

\noindent\textbf{Robin Berthier} is a research scientist at the University of Illinois at Urbana-Champaign, working with Prof. William H. Sanders. Robin graduated from the Reliability Engineering Department at the University of Maryland in 2009. His doctoral dissertation with Prof. Michel Cukier, and focused on the issue of honeypot sensors deployed on large networks. He introduced a new architecture to increase the scalability of high-interaction honeypots, and combined network datasets of different granularities to offer unique attack forensics capabilities. His current research interests include advanced intrusion detection systems and the security of critical infrastructures.

\begin{wrapfigure}{r}{0.17\textwidth}
  \begin{center}
    \includegraphics[width=0.14\textwidth]{./Figures/rakesh-bobba}
  \end{center}
\end{wrapfigure}

\noindent\textbf{Rakesh B. Bobba} is a Research Assistant Professor in the College of Engineering at the University of Illinois, Urbana-Champaign with appointments in Information Trust Institute and Electrical and Computer Engineering Department. His research interests are in the security of distributed and networked systems with a current focus on cyber-physical systems including critical infrastructures such as the power grid and cloud computing. He received M.S. and Ph.D. degrees in Electrical and Computer Engineering from the University of Maryland at College Park in 2007 and 2009, respectively.

\begin{wrapfigure}{r}{0.17\textwidth}
  \begin{center}
    \includegraphics[width=0.14\textwidth]{./Figures/bill-sanders}
  \end{center}
\end{wrapfigure}

\noindent\textbf{William H. Sanders} is a Donald Biggar Willett Professor of Engineering, the Interim Head of the Department of Electrical and Computer Engineering, and the Director of the Coordinated Science Laboratory (www.csl.illinois.edu) at the University of Illinois at Urbana-Champaign. He is a professor in the Department of Electrical and Computer Engineering and Affiliate Professor in the Department of Computer Science. He is a Fellow of the IEEE and the ACM, a past Chair of the IEEE Technical Committee on Fault-Tolerant Computing, and past Vice-Chair of the IFIP Working Group 10.4 on Dependable Computing. He was the founding Director of the Information Trust Institute (www.iti.illinois.edu) at Illinois.
